# Supplementary material for: Enhanced particle diffusion in fluctuating binary environments
Source: arXiv:2512.02776 ancillary file (2025-12-02)
Supplement: Supplementary file 1 [file SM.pdf]

# Supplemental Material: Enhanced particle diffusion in fluctuating binary environments


Fivos Perakis,[1,2] Takeshi Kawasaki,[3,4] and Shinji Saito[2,5]

[1] *Department of Physics, AlbaNova University Center, Stockholm University, S-106 91 Stockholm, Sweden*
[2] *Institute for Molecular Science, Myodaiji, Okazaki, Aichi 444-8585, Japan*
[3] *D3 Center, The University of Osaka, Toyonaka, Osaka, 560-0043, Japan*
[4] *Department of Physics, The University of Osaka, Toyonaka, Osaka, 560-0043, Japan*
[5] *The Graduate University for Advanced Studies (SOKENDAI), Myodaiji, Okazaki, Aichi 444-8585, Japan*


## UNITS AND NONDIMENSIONALIZATION

All simulations are performed in reduced units, where the relevant physical quantities are expressed relative to a fixed reference scale. Time is measured in units of the characteristic velocity–relaxation time $\tau_0 = m/\langle\gamma\rangle$, length in units of a reference distance $a$ (for instance, the probe diameter or cutoff distance used in $Q(t)$), and energy in units of $k_BT$. With these conventions, the Langevin equation [Eq. (1)] can be rewritten in dimensionless form without changing any of the parameters or numerical implementation used in the main text.

For clarity, we summarize the corresponding nondimensional variables:

$$r^* = \frac{r}{a}, \qquad t^* = \frac{t}{\tau_0}, \qquad v^* = \frac{v\,\tau_0}{a}, \qquad \gamma^*(t) = \frac{\gamma(t)}{\langle\gamma\rangle}.$$

Substituting into Eq. (1) gives the dimensionless update rule

$$\frac{dv^*}{dt^*} = -\,\gamma^*(t)\,v^* + \sqrt{2\,T^*\,\gamma^*(t)}\,\xi(t^*), \tag{S1}$$

where the dimensionless temperature parameter is

$$T^* = \frac{mk_BT}{a^2\langle\gamma\rangle^2}.$$

Here $T^*$ characterizes the relative strength of thermal to dissipative forces, while the time–dependent friction ratio $\gamma^*(t)$ introduces the stochastic switching dynamics between low– and high–friction states. We emphasize that in the simulations reported in the main text, $T$ and $\gamma(t)$ are treated as independent control parameters, and all results are expressed in the corresponding reduced units. The present formulation simply clarifies the underlying dimensional scales and provides a consistent basis for comparing with dimensional or experimental systems.

## MOBILITY FROM THE GREEN–KUBO RELATION

The particle mobility $\mu$ is computed from equilibrium trajectories using the Green–Kubo relation,

$$\mu = \frac{1}{k_BT}\int_0^\infty C_{vv}(t)\,dt, \qquad C_{vv}(t) = \langle v_x(t_0+t)\,v_x(t_0)\rangle, \tag{S2}$$

where $C_{vv}(t)$ is the velocity autocorrelation function (VACF) and $\langle\cdots\rangle$ denotes an average over time origins and trajectories. For isotropic motion, averaging over the $x$ and $y$ components yields the same result. The integral in Eq. (S2) is evaluated numerically using the trapezoidal rule up to the first zero crossing of $C_{vv}(t)$.

For consistency, the diffusion coefficient $D$ is obtained independently from the mean–squared displacement,

$$\langle\Delta r^2(t)\rangle = 4Dt \quad (t\to\infty), \tag{S3}$$

and compared to $k_BT\,\mu$ to verify the Einstein relation $D = k_BT\,\mu$, shown in Fig. S1. Panel (a) shows the VACF $C_{vv}(t)$ and panel (b) compares the diffusion constant $D$ from the MSD with $k_BT\,\mu$, demonstrating excellent agreement within numerical accuracy.

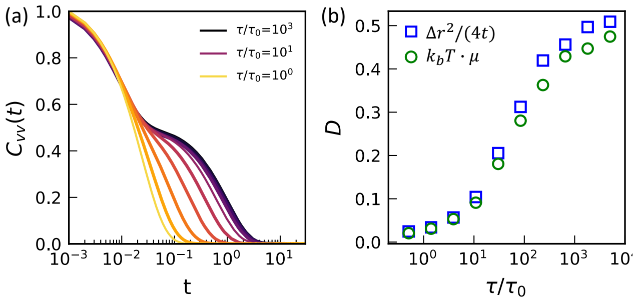


Fig. S1. (a) Velocity autocorrelation function (VACF) $C_{vv}(t)$; the shaded area equals $k_BT\,\mu$. (b) Einstein relation check: $D$ from the MSD versus $k_BT\,\widehat{\mu}_{\rm GK}$.

## INTERMEDIATE SCATTERING FUNCTION AND RELAXATION TIME

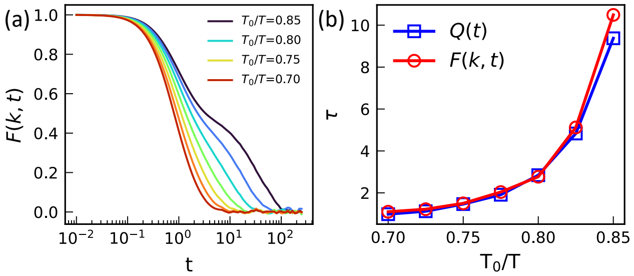


Fig. S2. (a) Self–intermediate scattering function $F(k, t)$ for several temperatures at fixed $\tau = 100$, showing a slower decay and more pronounced plateau upon cooling. (b) Structural relaxation time $\tau_\alpha$ extracted from the $F(k, t)$, displaying the same qualitative temperature dependence as obtained from the overlap function $Q(t)$.

To complement the overlap function analysis in the main text, we evaluate the self–intermediate scattering function (ISF), which provides an equivalent measure of single–particle relaxation in reciprocal space. The ISF is defined as

$$F(k,t) = \Big\langle \exp\big[i\,\mathbf{k}\cdot(\mathbf{r}(t_0+t) - \mathbf{r}(t_0))\big]\Big\rangle, \tag{S4}$$

where the average is taken over time origins $t_0$ and all simulated trajectories. The magnitude of the scattering vector is fixed at $k = 2\pi/a$, corresponding to the cut-off distance $a$ used in the overlap function $Q(t)$. The structural relaxation time $\tau_\alpha$ is extracted from the decay of $F_s(k, t)$ using the same threshold criterion applied to $Q(t)$, $F_s(k, \tau_\alpha) = 0.35$, which marks the crossover between the plateau and the final relaxation regime.

Figure S2 (a) shows $F_s(k, t)$ for several temperatures at fixed switching time $\tau = 100$, where cooling leads to a progressively slower decay and a more pronounced plateau. Panel (b) displays the corresponding relaxation times $\tau_\alpha$ as a function of temperature, revealing the same qualitative trend as observed from the overlap function.

## CHOICE OF THE OVERLAP CUTOFF PARAMETER $a$

The overlap function

$$Q(t) = \frac{1}{N}\sum_{i=1}^{N} w\big(|\mathbf{r}_i(t_0+t) - \mathbf{r}_i(t_0)|\big),$$

with $w(r) = 1$ if $r < a$ and 0 otherwise, depends on the cutoff $a$. This parameter selects which displacements are considered "correlated" and therefore influences both $Q(t)$ and its fluctuations $\chi_4(t)$.

If $a$ is too small, $Q(t)$ primarily reflects short-time vibrational motion, which is weakly correlated and leads to a rapid decay of $Q(t)$ with negligible $\chi_4(t)$. If $a$ is too large, a single particle may artificially "overlap" with multiple positions, inflating $Q(t)$.

For intermediate $a \sim 0.2$, $Q(t)$ develops a plateau and $\chi_4(t)$ exhibits a peak, indicating that correlated structural relaxation is probed [1]. Based on these considerations, we use $a = 0.2$ throughout this paper. Slight variations around this value do not qualitatively affect our conclusions.

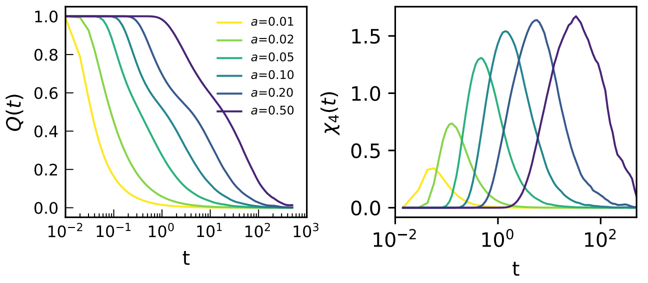


Fig. S3. Effect of the overlap cutoff parameter $a$. Overlap function $Q(t)$ (left) and four-point susceptibility $\chi_4(t)$ (right) at $T_0/T = 0.83$ and $P_s = 10^{-4}$ for several cutoff values $a$.


[1] N. Lačević, F. W. Starr, T. B. Schrøder, and S. C. Glotzer, The Journal of Chemical Physics **119**, 7372 (2003).
